# Supplementary material for: Function Space Diversity for Uncertainty Prediction via Repulsive Last-Layer Ensembles
Source: arXiv:2412.15758 source file (2024-12-20)
Supplement: Supplementary file 1 [file ensemble_head.tex]

\subsection{Ensemble head architecture} \label{app:ensemble_head_params}

In the following, we test the sensitivity of the network size for the repulsive ensemble heads.

We begin with the two moons toy example, as illustrated in Figure \ref{fig:ablation:network_size_toy}, and demonstrate that non-linear decision boundaries are necessary for the ensemble head to achieve diverse predictions far from the training data. The base network consists of three fully connected hidden layers with 128 neurons. There is no feature collapse in this scenario -- the input data is merely transformed to be linearly separable. In this case, nonlinear decision boundaries allow for uncertainty estimates that reflect the underlying data distribution.

Contrary to intuition, a repulsive ensemble consisting of linear layers performs well in the more complex task of OOD detection in image classification, without the need for additional nonlinearities.  For the image classification task, we use a Resnet-18 as the underlying feature extractor. The use of informative context points enables repulsive linear layers to significantly improve OOD detection. Enlarging the network size of the ensemble heads does not necessarily result in further improvements.
The base network is able to extract useful features for CIFAR10, but we still require informative context points to properly construct the linear classification layers, as shown in Figure \ref{fig:ablation:network_head}, where the use of CIFAR100 as context points performs comparably to full deep ensembles. Alternative context point choices do not noticeably improve the base network.
