# Supplementary material for: Function Space Diversity for Uncertainty Prediction via Repulsive Last-Layer Ensembles
Source: arXiv:2412.15758 source file (2024-12-20)
Supplement: Supplementary file 2 [file n_particles.tex]

%___________________________________________________________________________________
\subsection{Number of particles} \label{app:n_particles}

Lastly, we examine the number of particles, representing the number of ensemble head members (see Figure \ref{fig:ablation:num_particles}). We use a Resnet-18 as a base model and a repulsive ensemble head consisting of linear layers. Again, the best performance of MH-f-POVI is obtained by using unlabeled CIFAR100 samples as context points. We notice an initial rise in OOD detection as more particles are introduced, followed by a drop in ID accuracy and OOD detection. As the number of particles notably increases, the repulsion term prevails over the likelihood term in the loss function. Enforcing excessive diversity on context points that capture training data features results in decreased ID accuracy (see Figure \ref{fig:ablation:num_particles} for context points CIFAR100, and patches). Imposing diversity on random noise, on the other hand, has no effect on test accuracy. By reducing the strength of the repulsion term in the loss function through a scaling parameter (Figure \ref{fig:ablation:gamma}), we avoid the loss of ID accuracy. We show that for 5, 20, and 100 particles a decreasing weight of the repulsion term compared to the likelihood term mitigates ID performance degradation and improves OOD detection.
