# Supplementary material for: Function Space Diversity for Uncertainty Prediction via Repulsive Last-Layer Ensembles
Source: arXiv:2412.15758 source file (2024-12-20)
Supplement: Supplementary file 3 [file exp_spectral_norm.tex]

\pgfplotstableread[col sep=comma]{sections/graphs/OOD_CIFAR10/OOD_cifar10_auroc.csv}\tableOOD
\pgfplotstableread[col sep=comma]{sections/graphs/OOD_CIFAR10/ID_cifar10_accuracy.csv}\tableIDaccuracy
\pgfplotstableread[col sep=comma]{sections/graphs/OOD_CIFAR10/ID_cifar10_nll.csv}\tableIDnll
\pgfplotstableread[col sep=comma]{sections/graphs/OOD_CIFAR10/ID_cifar10_ece.csv}\tableIDece

\pgfplotstableread[col sep=comma]{sections/graphs/OOD_CIFAR10/OOD_cifar10_auroc_POVI_SGD.csv}\tableOODSGD
\pgfplotstableread[col sep=comma]{sections/graphs/OOD_CIFAR10/ID_cifar10_accuracy_POVI_SGD.csv}\tableIDaccuracySGD
\pgfplotstableread[col sep=comma]{sections/graphs/OOD_CIFAR10/ID_cifar10_nll_POVI_SGD.csv}\tableIDnllSGD
\pgfplotstableread[col sep=comma]{sections/graphs/OOD_CIFAR10/ID_cifar10_ece_POVI_SGD.csv}\tableIDeceSGD

\pgfplotstableread[col sep=comma]{sections/graphs/OOD_CIFAR10/OOD_cifar10_auroc_POVI_kde_WGD.csv}\tableOODWGD
\pgfplotstableread[col sep=comma]{sections/graphs/OOD_CIFAR10/ID_cifar10_accuracy_POVI_kde_WGD.csv}\tableIDaccuracyWGD
\pgfplotstableread[col sep=comma]{sections/graphs/OOD_CIFAR10/ID_cifar10_nll_POVI_kde_WGD.csv}\tableIDnllWGD
\pgfplotstableread[col sep=comma]{sections/graphs/OOD_CIFAR10/ID_cifar10_ece_POVI_kde_WGD.csv}\tableIDeceWGD

\pgfplotstableread[col sep=comma]{sections/graphs/OOD_CIFAR10/OOD_cifar10_auroc_POVI_kde_f_WGD_coll_cifar100.csv}\tableOODcifar
\pgfplotstableread[col sep=comma]{sections/graphs/OOD_CIFAR10/ID_cifar10_accuracy_POVI_kde_f_WGD_coll_cifar100.csv}\tableIDaccuracycifar
\pgfplotstableread[col sep=comma]{sections/graphs/OOD_CIFAR10/ID_cifar10_nll_POVI_kde_f_WGD_coll_cifar100.csv}\tableIDnllcifar
\pgfplotstableread[col sep=comma]{sections/graphs/OOD_CIFAR10/ID_cifar10_ece_POVI_kde_f_WGD_coll_cifar100.csv}\tableIDececifar

\pgfplotstableread[col sep=comma]{sections/graphs/OOD_CIFAR10/OOD_cifar10_auroc_POVI_kde_f_WGD_coll_tinyimagenet.csv}\tableOODFtiny
\pgfplotstableread[col sep=comma]{sections/graphs/OOD_CIFAR10/ID_cifar10_accuracy_POVI_kde_f_WGD_coll_tinyimagenet.csv}\tableIDaccuracyFtiny
\pgfplotstableread[col sep=comma]{sections/graphs/OOD_CIFAR10/ID_cifar10_nll_POVI_kde_f_WGD_coll_tinyimagenet.csv}\tableIDnllFtiny
\pgfplotstableread[col sep=comma]{sections/graphs/OOD_CIFAR10/ID_cifar10_ece_POVI_kde_f_WGD_coll_tinyimagenet.csv}\tableIDeceFtiny

\pgfplotstableread[col sep=comma]{sections/graphs/OOD_CIFAR10/OOD_cifar10_auroc_POVI_kde_f_WGD_coll_texture.csv}\tableOODFtext
\pgfplotstableread[col sep=comma]{sections/graphs/OOD_CIFAR10/ID_cifar10_accuracy_POVI_kde_f_WGD_coll_texture.csv}\tableIDaccuracyFtext
\pgfplotstableread[col sep=comma]{sections/graphs/OOD_CIFAR10/ID_cifar10_nll_POVI_kde_f_WGD_coll_texture.csv}\tableIDnllFtext
\pgfplotstableread[col sep=comma]{sections/graphs/OOD_CIFAR10/ID_cifar10_ece_POVI_kde_f_WGD_coll_texture.csv}\tableIDeceFtext

\pgfplotstableread[col sep=comma]{sections/graphs/OOD_CIFAR10/OOD_cifar10_auroc_POVI_patches_std_16.csv}\tableOODPatchsixteen
\pgfplotstableread[col sep=comma]{sections/graphs/OOD_CIFAR10/ID_cifar10_accuracy_POVI_patches_std_16.csv}\tableIDaccuracyPatchsixteen
\pgfplotstableread[col sep=comma]{sections/graphs/OOD_CIFAR10/ID_cifar10_nll_POVI_patches_std_16.csv}\tableIDnllPatchsixteen
\pgfplotstableread[col sep=comma]{sections/graphs/OOD_CIFAR10/ID_cifar10_ece_POVI_patches_std_16.csv}\tableIDecePatchsixteen

\pgfplotstableread[col sep=comma]{sections/graphs/OOD_CIFAR10/OOD_cifar10_auroc_POVI_patches_std_32.csv}\tableOODPatchthirtytwo
\pgfplotstableread[col sep=comma]{sections/graphs/OOD_CIFAR10/ID_cifar10_accuracy_POVI_patches_std_32.csv}\tableIDaccuracyPatchthirtytwo
\pgfplotstableread[col sep=comma]{sections/graphs/OOD_CIFAR10/ID_cifar10_nll_POVI_patches_std_32.csv}\tableIDnllPatchthirtytwo
\pgfplotstableread[col sep=comma]{sections/graphs/OOD_CIFAR10/ID_cifar10_ece_POVI_patches_std_32.csv}\tableIDecePatchthirtytwo

\pgfplotstableread[col sep=comma]{sections/graphs/OOD_CIFAR10/OOD_cifar10_auroc_POVI_patches_std_8.csv}\tableOODPatcheight
\pgfplotstableread[col sep=comma]{sections/graphs/OOD_CIFAR10/ID_cifar10_accuracy_POVI_patches_std_8.csv}\tableIDaccuracyPatcheight
\pgfplotstableread[col sep=comma]{sections/graphs/OOD_CIFAR10/ID_cifar10_nll_POVI_patches_std_8.csv}\tableIDnllPatcheight
\pgfplotstableread[col sep=comma]{sections/graphs/OOD_CIFAR10/ID_cifar10_ece_POVI_patches_std_8.csv}\tableIDecePatcheight

\renewcommand{\fetchAndStore}[4]{%
    \pgfplotstablegetelem{#1}{#2}\of{#3}
    \expandafter\xdef\csname #2Mean#1#4\endcsname{\pgfplotsretval}
    \pgfplotstablegetelem{#1}{#2_std}\of{#3}
    \expandafter\xdef\csname #2Std#1#4\endcsname{\pgfplotsretval}
}

% Using foreach to iterate over methods and intensities
\foreach \method in {softmax,logits,logits_GMM,softmax_laplace_MI,softmax_SNGP_PE,softmax_en_PE,softmax_en_MI} {
    \foreach \intensity in {0,1,2,3,4,5} { % Adjust index for 0-based indexing in CSV
        \fetchAndStore{\intensity}{\method}{\tableOOD}{OOD}
    }
}

\foreach \method in {softmax,logits,logits_GMM,softmax_laplace_MI,softmax_SNGP_PE,softmax_en_PE,softmax_en_MI} {
    \fetchAndStore{0}{\method}{\tableIDaccuracy}{accuracy}
    \fetchAndStore{0}{\method}{\tableIDnll}{nll}
    \fetchAndStore{0}{\method}{\tableIDece}{ece}
}

% Using foreach to iterate over methods and intensities
\foreach \method in {softmax_POVI_MI} {
    \foreach \intensity in {0,1,2,3,4,5} { % Adjust index for 0-based indexing in CSV
        \fetchAndStore{\intensity}{\method}{\tableOODSGD}{OODSGD}
        \fetchAndStore{\intensity}{\method}{\tableOODWGD}{OODWGD}
        \fetchAndStore{\intensity}{\method}{\tableOODFtiny}{OODFtiny}
        \fetchAndStore{\intensity}{\method}{\tableOODcifar}{OODcifar}
        \fetchAndStore{\intensity}{\method}{\tableOODFtext}{OODFtext}
        \fetchAndStore{\intensity}{\method}{\tableOODPatchsixteen}{OODPatchsixteen}
        \fetchAndStore{\intensity}{\method}{\tableOODPatchthirtytwo}{OODPatchthirtytwo}
        \fetchAndStore{\intensity}{\method}{\tableOODPatcheight}{OODPatcheight}
    }
}
\foreach \method in {softmax_POVI_MI} {
    \fetchAndStore{0}{\method}{\tableIDaccuracySGD}{accuracySGD}
    \fetchAndStore{0}{\method}{\tableIDnllSGD}{nllSGD}
    \fetchAndStore{0}{\method}{\tableIDeceSGD}{eceSGD}

    \fetchAndStore{0}{\method}{\tableIDaccuracyWGD}{accuracyWGD}
    \fetchAndStore{0}{\method}{\tableIDnllWGD}{nllWGD}
    \fetchAndStore{0}{\method}{\tableIDeceWGD}{eceWGD}
    
    \fetchAndStore{0}{\method}{\tableIDaccuracycifar}{accuracycifar}
    \fetchAndStore{0}{\method}{\tableIDnllcifar}{nllcifar}
    \fetchAndStore{0}{\method}{\tableIDececifar}{ececifar}
    
    \fetchAndStore{0}{\method}{\tableIDaccuracyFtiny}{accuracyFtiny}
    \fetchAndStore{0}{\method}{\tableIDnllFtiny}{nllFtiny}
    \fetchAndStore{0}{\method}{\tableIDeceFtiny}{eceFtiny}
    
    \fetchAndStore{0}{\method}{\tableIDaccuracyFtext}{accuracyFtext}
    \fetchAndStore{0}{\method}{\tableIDnllFtext}{nllFtext}
    \fetchAndStore{0}{\method}{\tableIDeceFtext}{eceFtext}

    \fetchAndStore{0}{\method}{\tableIDaccuracyPatchsixteen}{accuracyPatchsixteen}
    \fetchAndStore{0}{\method}{\tableIDnllPatchsixteen}{nllPatchsixteen}
    \fetchAndStore{0}{\method}{\tableIDecePatchsixteen}{ecePatchsixteen}
    
    \fetchAndStore{0}{\method}{\tableIDaccuracyPatchthirtytwo}{accuracyPatchthirtytwo}
    \fetchAndStore{0}{\method}{\tableIDnllPatchthirtytwo}{nllPatchthirtytwo}
    \fetchAndStore{0}{\method}{\tableIDecePatchthirtytwo}{ecePatchthirtytwo}
    
    \fetchAndStore{0}{\method}{\tableIDaccuracyPatcheight}{accuracyPatcheight}
    \fetchAndStore{0}{\method}{\tableIDnllPatcheight}{nllPatcheight}
    \fetchAndStore{0}{\method}{\tableIDecePatcheight}{ecePatcheight}
}

% Please add the following required packages to your document preamble:
% \usepackage{multirow}
% \usepackage{graphicx}
\begin{table}[]
\centering
\caption{}
\label{tab:my-table}
\resizebox{\columnwidth}{!}{%
\begin{tabular}{lclccccccccc}
\hline
\multicolumn{3}{l}{~~~\textbf{Ablations}} &
  \multirow{2}{*}{\textsc{Acc.} $\uparrow$ [\%]} &
  \multirow{2}{*}{\textsc{NLL} $\downarrow$ [\%]} &
  \multirow{2}{*}{\textsc{ECE} $\downarrow$ [\%]} &
  \multicolumn{6}{c}{\textsc{OOD} \textsc{Auroc} $\uparrow$ [\%]} \\ \cline{1-3} \cline{7-12} 
 &
  \multicolumn{1}{l}{SN} &
  Method &
   &
   &
   &
  \textit{Cifar100} &
  \textit{TinyIm.} &
  \textit{Places365} &
  \textit{Texture} &
  \textit{SVHN} &
  \textit{FakeData} \\ \hline
\multirow{10}{*}{\rotatebox[origin=c]{90}{Resnet-18}} & 
        \multirow{5}{*}{\cmark} &
  MAP &
  ${\csname softmaxMean0accuracy\endcsname _{\pm \csname softmaxStd0accuracy\endcsname}}$ &
  ${\csname softmaxMean0nll\endcsname _{\pm \csname softmaxStd0nll\endcsname}}$ &
  ${\csname softmaxMean0ece\endcsname _{\pm \csname softmaxStd0ece\endcsname}}$ &
  ${\csname softmaxMean0OOD\endcsname _{\pm \csname softmaxStd0OOD\endcsname}}$ &
  ${\csname softmaxMean1OOD\endcsname _{\pm \csname softmaxStd1OOD\endcsname}}$ &
  ${\csname softmaxMean2OOD\endcsname _{\pm \csname softmaxStd2OOD\endcsname}}$ &
  ${\csname softmaxMean3OOD\endcsname _{\pm \csname softmaxStd3OOD\endcsname}}$ &
  ${\csname softmaxMean4OOD\endcsname _{\pm \csname softmaxStd4OOD\endcsname}}$ &
  ${\csname softmaxMean5OOD\endcsname _{\pm \csname softmaxStd5OOD\endcsname}}$ \\ \cline{3-12} 
 &
   &
  DDU &
  ${\csname softmaxMean0accuracy\endcsname _{\pm \csname softmaxStd0accuracy\endcsname}}$ &
  ${\csname softmaxMean0nll\endcsname _{\pm \csname softmaxStd0nll\endcsname}}$ &
  ${\csname softmaxMean0ece\endcsname _{\pm \csname softmaxStd0ece\endcsname}}$ &
  ${\csname logits_GMMMean0OOD\endcsname _{\pm \csname logits_GMMStd0OOD\endcsname}}$ &
  ${\csname logits_GMMMean1OOD\endcsname _{\pm \csname logits_GMMStd1OOD\endcsname}}$ &
  ${\csname logits_GMMMean2OOD\endcsname _{\pm \csname logits_GMMStd2OOD\endcsname}}$ &
  ${\csname logits_GMMMean3OOD\endcsname _{\pm \csname logits_GMMStd3OOD\endcsname}}$ &
  ${\csname logits_GMMMean4OOD\endcsname _{\pm \csname logits_GMMStd4OOD\endcsname}}$ &
  $\mathbf{\csname logits_GMMMean5OOD\endcsname _{\pm \csname logits_GMMStd5OOD\endcsname}}$ \\
 &
   &
  LL-Laplace &
  ${\csname softmax_laplace_MIMean0accuracy\endcsname _{\pm \csname softmax_laplace_MIStd0accuracy\endcsname}}$ &
  ${\csname softmax_laplace_MIMean0nll\endcsname _{\pm \csname softmax_laplace_MIStd0nll\endcsname}}$ &
  ${\csname softmax_laplace_MIMean0ece\endcsname _{\pm \csname softmax_laplace_MIStd0ece\endcsname}}$ &
  ${\csname softmax_laplace_MIMean0OOD\endcsname _{\pm \csname softmax_laplace_MIStd0OOD\endcsname}}$ &
  ${\csname softmax_laplace_MIMean1OOD\endcsname _{\pm \csname softmax_laplace_MIStd1OOD\endcsname}}$ &
  ${\csname softmax_laplace_MIMean2OOD\endcsname _{\pm \csname softmax_laplace_MIStd2OOD\endcsname}}$ &
  ${\csname softmax_laplace_MIMean3OOD\endcsname _{\pm \csname softmax_laplace_MIStd3OOD\endcsname}}$ &
  ${\csname softmax_laplace_MIMean4OOD\endcsname _{\pm \csname softmax_laplace_MIStd4OOD\endcsname}}$ &
  ${\csname softmax_laplace_MIMean5OOD\endcsname _{\pm \csname softmax_laplace_MIStd5OOD\endcsname}}$ \\ \cline{3-12} 
 &
   &
  \gls{LLPOVI} \emph{(ours)} &
  ${\csname softmax_POVI_MIMean0accuracySGD\endcsname _{\pm \csname softmax_POVI_MIStd0accuracySGD\endcsname}}$ &
  ${\csname softmax_POVI_MIMean0nllSGD\endcsname _{\pm \csname softmax_POVI_MIStd0nllSGD\endcsname}}$ &
  ${\csname softmax_POVI_MIMean0eceSGD\endcsname _{\pm \csname softmax_POVI_MIStd0eceSGD\endcsname}}$ &
  ${\csname softmax_POVI_MIMean0OODSGD\endcsname _{\pm \csname softmax_POVI_MIStd0OODSGD\endcsname}}$ &
  ${\csname softmax_POVI_MIMean1OODSGD\endcsname _{\pm \csname softmax_POVI_MIStd1OODSGD\endcsname}}$ &
  ${\csname softmax_POVI_MIMean2OODSGD\endcsname _{\pm \csname softmax_POVI_MIStd2OODSGD\endcsname}}$ &
  ${\csname softmax_POVI_MIMean3OODSGD\endcsname _{\pm \csname softmax_POVI_MIStd3OODSGD\endcsname}}$ &
  ${\csname softmax_POVI_MIMean4OODSGD\endcsname _{\pm \csname softmax_POVI_MIStd4OODSGD\endcsname}}$ &
  ${\csname softmax_POVI_MIMean5OODSGD\endcsname _{\pm \csname softmax_POVI_MIStd5OODSGD\endcsname}}$ \\
 &
   &
  \gls{fLLPOVI} \emph{(ours)} &
  ${\csname softmax_POVI_MIMean0accuracySGD\endcsname _{\pm \csname softmax_POVI_MIStd0accuracySGD\endcsname}}$ &
  ${\csname softmax_POVI_MIMean0nllSGD\endcsname _{\pm \csname softmax_POVI_MIStd0nllSGD\endcsname}}$ &
  ${\csname softmax_POVI_MIMean0eceSGD\endcsname _{\pm \csname softmax_POVI_MIStd0eceSGD\endcsname}}$ &
  ${\csname softmax_POVI_MIMean0OODSGD\endcsname _{\pm \csname softmax_POVI_MIStd0OODSGD\endcsname}}$ &
  ${\csname softmax_POVI_MIMean1OODSGD\endcsname _{\pm \csname softmax_POVI_MIStd1OODSGD\endcsname}}$ &
  ${\csname softmax_POVI_MIMean2OODSGD\endcsname _{\pm \csname softmax_POVI_MIStd2OODSGD\endcsname}}$ &
  ${\csname softmax_POVI_MIMean3OODSGD\endcsname _{\pm \csname softmax_POVI_MIStd3OODSGD\endcsname}}$ &
  ${\csname softmax_POVI_MIMean4OODSGD\endcsname _{\pm \csname softmax_POVI_MIStd4OODSGD\endcsname}}$ &
  ${\csname softmax_POVI_MIMean5OODSGD\endcsname _{\pm \csname softmax_POVI_MIStd5OODSGD\endcsname}}$ \\ \cline{2-12} 
 &
  \multirow{5}{*}{\xmark} &
  MAP &
  ${\csname softmaxMean0accuracy\endcsname _{\pm \csname softmaxStd0accuracy\endcsname}}$ &
  ${\csname softmaxMean0nll\endcsname _{\pm \csname softmaxStd0nll\endcsname}}$ &
  ${\csname softmaxMean0ece\endcsname _{\pm \csname softmaxStd0ece\endcsname}}$ &
  ${\csname softmaxMean0OOD\endcsname _{\pm \csname softmaxStd0OOD\endcsname}}$ &
  ${\csname softmaxMean1OOD\endcsname _{\pm \csname softmaxStd1OOD\endcsname}}$ &
  ${\csname softmaxMean2OOD\endcsname _{\pm \csname softmaxStd2OOD\endcsname}}$ &
  ${\csname softmaxMean3OOD\endcsname _{\pm \csname softmaxStd3OOD\endcsname}}$ &
  ${\csname softmaxMean4OOD\endcsname _{\pm \csname softmaxStd4OOD\endcsname}}$ &
  ${\csname softmaxMean5OOD\endcsname _{\pm \csname softmaxStd5OOD\endcsname}}$ \\ \cline{3-12} 
 &
   &
  DDU &
  ${\csname softmaxMean0accuracy\endcsname _{\pm \csname softmaxStd0accuracy\endcsname}}$ &
  ${\csname softmaxMean0nll\endcsname _{\pm \csname softmaxStd0nll\endcsname}}$ &
  ${\csname softmaxMean0ece\endcsname _{\pm \csname softmaxStd0ece\endcsname}}$ &
  ${\csname logits_GMMMean0OOD\endcsname _{\pm \csname logits_GMMStd0OOD\endcsname}}$ &
  ${\csname logits_GMMMean1OOD\endcsname _{\pm \csname logits_GMMStd1OOD\endcsname}}$ &
  ${\csname logits_GMMMean2OOD\endcsname _{\pm \csname logits_GMMStd2OOD\endcsname}}$ &
  ${\csname logits_GMMMean3OOD\endcsname _{\pm \csname logits_GMMStd3OOD\endcsname}}$ &
  ${\csname logits_GMMMean4OOD\endcsname _{\pm \csname logits_GMMStd4OOD\endcsname}}$ &
  $\mathbf{\csname logits_GMMMean5OOD\endcsname _{\pm \csname logits_GMMStd5OOD\endcsname}}$ \\
 &
   &
  LL-Laplace &
  ${\csname softmax_laplace_MIMean0accuracy\endcsname _{\pm \csname softmax_laplace_MIStd0accuracy\endcsname}}$ &
  ${\csname softmax_laplace_MIMean0nll\endcsname _{\pm \csname softmax_laplace_MIStd0nll\endcsname}}$ &
  ${\csname softmax_laplace_MIMean0ece\endcsname _{\pm \csname softmax_laplace_MIStd0ece\endcsname}}$ &
  ${\csname softmax_laplace_MIMean0OOD\endcsname _{\pm \csname softmax_laplace_MIStd0OOD\endcsname}}$ &
  ${\csname softmax_laplace_MIMean1OOD\endcsname _{\pm \csname softmax_laplace_MIStd1OOD\endcsname}}$ &
  ${\csname softmax_laplace_MIMean2OOD\endcsname _{\pm \csname softmax_laplace_MIStd2OOD\endcsname}}$ &
  ${\csname softmax_laplace_MIMean3OOD\endcsname _{\pm \csname softmax_laplace_MIStd3OOD\endcsname}}$ &
  ${\csname softmax_laplace_MIMean4OOD\endcsname _{\pm \csname softmax_laplace_MIStd4OOD\endcsname}}$ &
  ${\csname softmax_laplace_MIMean5OOD\endcsname _{\pm \csname softmax_laplace_MIStd5OOD\endcsname}}$ \\  \cline{3-12} 
 &
   &
  \gls{LLPOVI} \emph{(ours)} &
  ${\csname softmax_POVI_MIMean0accuracySGD\endcsname _{\pm \csname softmax_POVI_MIStd0accuracySGD\endcsname}}$ &
  ${\csname softmax_POVI_MIMean0nllSGD\endcsname _{\pm \csname softmax_POVI_MIStd0nllSGD\endcsname}}$ &
  ${\csname softmax_POVI_MIMean0eceSGD\endcsname _{\pm \csname softmax_POVI_MIStd0eceSGD\endcsname}}$ &
  ${\csname softmax_POVI_MIMean0OODSGD\endcsname _{\pm \csname softmax_POVI_MIStd0OODSGD\endcsname}}$ &
  ${\csname softmax_POVI_MIMean1OODSGD\endcsname _{\pm \csname softmax_POVI_MIStd1OODSGD\endcsname}}$ &
  ${\csname softmax_POVI_MIMean2OODSGD\endcsname _{\pm \csname softmax_POVI_MIStd2OODSGD\endcsname}}$ &
  ${\csname softmax_POVI_MIMean3OODSGD\endcsname _{\pm \csname softmax_POVI_MIStd3OODSGD\endcsname}}$ &
  ${\csname softmax_POVI_MIMean4OODSGD\endcsname _{\pm \csname softmax_POVI_MIStd4OODSGD\endcsname}}$ &
  ${\csname softmax_POVI_MIMean5OODSGD\endcsname _{\pm \csname softmax_POVI_MIStd5OODSGD\endcsname}}$ \\
 &
   &
  \gls{fLLPOVI} \emph{(ours)} &
  ${\csname softmax_POVI_MIMean0accuracySGD\endcsname _{\pm \csname softmax_POVI_MIStd0accuracySGD\endcsname}}$ &
  ${\csname softmax_POVI_MIMean0nllSGD\endcsname _{\pm \csname softmax_POVI_MIStd0nllSGD\endcsname}}$ &
  ${\csname softmax_POVI_MIMean0eceSGD\endcsname _{\pm \csname softmax_POVI_MIStd0eceSGD\endcsname}}$ &
  ${\csname softmax_POVI_MIMean0OODSGD\endcsname _{\pm \csname softmax_POVI_MIStd0OODSGD\endcsname}}$ &
  ${\csname softmax_POVI_MIMean1OODSGD\endcsname _{\pm \csname softmax_POVI_MIStd1OODSGD\endcsname}}$ &
  ${\csname softmax_POVI_MIMean2OODSGD\endcsname _{\pm \csname softmax_POVI_MIStd2OODSGD\endcsname}}$ &
  ${\csname softmax_POVI_MIMean3OODSGD\endcsname _{\pm \csname softmax_POVI_MIStd3OODSGD\endcsname}}$ &
  ${\csname softmax_POVI_MIMean4OODSGD\endcsname _{\pm \csname softmax_POVI_MIStd4OODSGD\endcsname}}$ &
  ${\csname softmax_POVI_MIMean5OODSGD\endcsname _{\pm \csname softmax_POVI_MIStd5OODSGD\endcsname}}$  \\ \bottomrule
\end{tabular}%
}
\end{table}
